# Supplementary material for: Operator product expansion for the non-local gluon condensate
Source: arXiv:2103.09478 ancillary file (2021-05-13)
Supplement: Supplementary file 1 [file README_GG.pdf]

Files `zCF.mres`, `xCF.mres`, `sCF.mres`, `tCF.mres`, `ad.mres` and `rc.mres` contain the MATHEMATICA versions (in general covariant gauge and for general gauge group) of the results given in a shortened form in Section 4 of V. M. Braun, K. G. Chetyrkin and B. Kniehl “Operator product expansion for the non-local gluon condensate”.

**Notations:**

`z3`, `z5` stand for the values of the Riemann zeta-function with  $z3 = \zeta_3 = 1.2020569\dots$ ,  $z5 = \zeta_5 = 1.0369278\dots$ .

`cf` =  $C_F$  and `ca` =  $C_A$  are the quadratic Casimir operators of the quark  $[T^a T^a]_{ij} = C_F \delta_{ij}$  and the adjoint  $[C^a C^a]_{bd} = C_A \delta_{bd}$ ,  $(C^a)_{bc} = -if^{abc}$  representations of the Lie algebra, `ng` and `dR` are dimensions of the adjoint (gluon) and quark representations of the gauge group, `nf` stands for the number of quark flavors and `tr` =  $T_f$  refers to the trace normalization  $\text{tr}(T^a T^b) = T_f \delta^{ab}$ .

Finally, `om` =  $\omega = pv$ , `vv` =  $v \cdot v$ , `m2q` =  $\sum_i m_i^2$ , `m4di` =  $\sum_i m_i^4$ , `m4ns` =  $\sum_{i \neq j} m_i^2 m_j^2$ , and

$$\text{tLn} = \ln \frac{\mu}{-2\omega}, \text{sLn} = \ln \frac{\mu}{2\omega}, \text{xLn} = \ln \left( \frac{\mu i t e^{\gamma_E}}{2} \right), \text{zLn} = \ln \left( \frac{\mu z e^{\gamma_E}}{2} \right),$$

with  $\gamma_E = 0.577216\dots$ , being the Euler constant appearing in the expansion of the Gamma function

$$\Gamma(1 + \epsilon) = 1 - \gamma_E \epsilon + \mathcal{O}(\epsilon^2).$$

File `zCF.mres` contains expressions

`zPimq4tt`, `zC02tt`, `zC01tt`, `zPimq4pt`, `zC02pt`, `zC01pt` which correspond to the functions  $\Pi_{\perp\perp}^{m^4}(z)$ ,  $C_2^{\perp\perp}(z)$ ,  $\mathbb{C}_1^{\perp\perp} \equiv \frac{g^2}{12} C_1^{\perp\perp}$ ,  $\Pi_{\parallel\perp}^{m^4}(z)$ ,  $C_2^{\parallel\perp}(z)$  and  $\mathbb{C}_1^{\parallel\perp} \equiv \frac{g^2}{12} C_1^{\parallel\perp}$ , as defined in eqs (2.6) and (2.5) of the paper.

For the case of the time-like vector  $v$  (with  $v^2 = 1$ ) the same functions depend on the variable `t` and the combination `xLn`. They are encoded as

`xPimq4tt`, `xC02tt`, `xC01tt`, `xPimq4pt`, `xC02pt`, `xC01pt`,  
and put into the file `xCF.mres`.

Finally, the momentum space versions of the same CFs are labeled as

`sPimq4tt`, `sC02tt`, `sC01tt`, `sPimq4pt`, `sC02pt`, `sC01pt`  
(space-like vector  $v$ ,  $v^2 = -1$ ) and  
`tPimq4tt`, `tC02tt`, `tC01tt`, `tPimq4pt`, `tC02pt`, `tC01pt`

(time-like vector  $v$ ,  $v^2 = 1$ ) and put into the files `sCF.mres` and `tCF.mres` respectively.

Note, that have used a symbol `Im1`  $\equiv i \equiv \sqrt{-1}$  instead of the Mathematica symbol `I` for the the imaginary unit. A symbol `x` is introduced as a convenient label in the relation (see eq. (3.43) of [1])

$$\text{tLn} \rightarrow \text{sLn} + \text{x} * (\text{Im1} * \text{Pi}/2). \tag{1}$$

Within a Mathematica session it can always be removed by saying

$$\text{x} = 1;$$

File `rc.mres` contains the renormalization constants `Zpt` and `Ztt` to the 3-loop accuracy.  
 File `ad.mres` contains the QCD  $\beta$ -function `=be`, as well as the ADs

$$\text{gm}=\gamma_m, \quad \text{g011}=\gamma_{11}, \quad \text{g012}=\gamma_{12} \quad \text{g0di}=\gamma_0^{\text{di}} \quad \text{g0nd}=\gamma_0^{\text{nd}} \quad \text{gtt}=\gamma_{\perp\perp}, \quad \text{gpt}=\gamma_{\parallel\perp}$$

(all to the 3-loop accuracy).

### Bibliography notes:

Some of results given in the auxiliary files were originally obtained by other authors and have been included by us for completeness.

The VEV of the gluon off-light-cone operator  $\mathbb{G}_{\mu\nu\alpha\beta}$  in two loops was found in [2] and the corresponding 1-loop ADs first computed in [3, 4]. The anomalous dimension of the vacuum energy was taken from [5, 6, 7]. The 3-loop  $\beta$ -function and the quark mass AD are well-known since long [8, 9, 10].

### References

- [1] V. Braun, K. Chetyrkin and B. Kniehl, *Renormalization of parton quasi-distributions beyond the leading order: spacelike vs. timelike*, *JHEP* **07** (2020) 161, [2004.01043].
- [2] M. Eidemuller and M. Jamin, *QCD field strength correlator at the next-to-leading order*, *Phys. Lett.* **B416** (1998) 415–420, [hep-ph/9709419].
- [3] H. Dorn and E. Wiczeorek, *Renormalization and Short Distance Properties of String Type Equations in QCD*, *Z. Phys.* **C9** (1981) 49.
- [4] H. Dorn, D. Robaschik and E. Wiczeorek, *Renormalization and short distance properties of gauge invariant gluonium and hadron operators*, *Annalen Phys.* **40** (1983) 166.
- [5] V. P. Spiridonov and K. G. Chetyrkin, *Nonleading mass corrections and renormalization of the operators  $m\bar{\psi}\psi$  and  $G_{\mu\nu}^2$* , *Sov. J. Nucl. Phys.* **47** (1988) 522–527.
- [6] K. G. Chetyrkin and J. H. Kuhn, *Quartic mass corrections to  $R(\text{had})$* , *Nucl. Phys. B* **432** (1994) 337–350, [hep-ph/9406299].
- [7] P. A. Baikov and K. G. Chetyrkin, *QCD vacuum energy in 5 loops*, *PoS RADCOR2017* (2018) 025.
- [8] O. V. Tarasov, A. A. Vladimirov and A. Y. Zharkov, *The Gell-Mann-Low function of QCD in the three loop approximation*, *Phys. Lett.* **B93** (1980) 429–432.
- [9] O. V. Tarasov, *Anomalous dimensions of quark masses in the three-loop approximation*, 1910.12231.
- [10] S. A. Larin and J. A. M. Vermaseren, *The Three loop QCD Beta function and anomalous dimensions*, *Phys. Lett.* **B303** (1993) 334–336, [hep-ph/9302208].
